# Supplementary material for: Boosting Binary Masks for Multi-Domain Learning through Affine Transformations
Source: arXiv:2103.13894 source file (2021-03-25)
Supplement: Supplementary file 1 [file ablation.tex]

In this section we extend the ablation study of the main paper (Table~5) by including 2 additional settings (Full with no bias, \ie with $k_1=0$, and Full with $k_2=0$), and by considering an additional architecture, \ie DenseNet-121. Settings involving learning also $k_0$ were not considered, for the reason mentioned in the main paper, \ie having task-specific batch-normalization parameters allows us to neglect an additional degree of freedom. The surrogate function we use is the identity function $\tilde{h}(x)=x$, unless otherwise stated (\ie \textit{with Sigmoid}). The analysis is shown in Table \ref{tab:ablation-res} and repeated for the DenseNet-121 architecture in Table \ref{tab:ablation-dense}.

We have reported in Table~\ref{tab:ablation-res} the ablation study presented in Table~5 of the main paper for the sake of easier comparison and we have added two entries, namely \emph{Full, no bias} and \emph{Full, no $k_2$}, which we are going to comment, while we refer to the main paper for the rest of the study. As we can see, there is a clear drop in performance in various scenarios (\eg CUBS, Cars) when we set $k_1=0$ or $k_2=0$, thus highlighting the importance of those components. We also notice that a similar drop was affecting our \emph{Simple} version when bias was omitted. 

Table \ref{tab:ablation-dense} shows the ablation with DenseNet-121. We can draw in general similar conclusions to the ones of ResNet-50. Adding task-specific BN layers increases the performances of Piggyback, without additional gains obtained when a bias term is considered. Similarly, for our models, no significant gain is obtained when a sigmoidal surrogate function is used or when a channel-wise bias term is considered.
We also note that, as opposed to ResNet-50, setting $k_1$ to zero degrades the performance only in 1 out of 5 datasets (\ie CUBS) while the other 4 are not affected, showing that the effectiveness of different components of the model is also dependent on the architecture used.

Noticeable, the full versions with $k_2=0$ suffer a large decrease in performances in almost all settings (\eg ResNet-50 Flowers from 96.7\% to 91.0\%), showing that the component that brings the largest benefits to our algorithm is the addition of the binary mask itself scaled by $k_2$ (\ie $k_2 \cdot \mat M$). This explains also the reason why the simple version achieves a performance similar to the full version of our model. We finally note that there is a limited contribution brought by the standard Piggyback component (\ie $k_1\cdot \mat W\circ \mat M$), compared to the new components that we have introduced in the transformation.
\begin{table}[t]
			\caption{Impact of the parameters $k_0$, $k_1$, $k_2$ and $k_3$ of our model using the ResNet-50 architectures in the ImageNet-to-Sketch scenario. \ding{51} denotes a learned parameter, while~$^*$ denotes \cite{mallya2018piggyback} obtained as a special case of our model.} 

		\vspace{5pt}
		\centering
		\begin{tabular}{ l | c | c | c | c | c | c | c | c | c |  } 
        Method &$k_0$ &$k_1$ & $k_2$&$k_3$& CUBS & CARS & Flowers & WikiArt & Sketch\\
         \hline
Piggyback \cite{mallya2018piggyback}&0&0&0&1&80.4&88.1&93.6&73.4&79.4\\
\hline
Piggyback$^*$ 
&0&0&0&1&80.4&87.8&93.1&72.5&78.6\\ 
Piggyback$^*$ with BN & 0&0&0&1 &82.1&90.6&95.2&74.1&79.4\\ 
Piggyback$^*$ with BN
&0&\ding{51}&0&1&81.9&89.9&94.8&73.7&79.9\\ 
        Ours (Simple, no bias)
&1&0&\ding{51}&0&80.8&90.3&96.1&73.5&80.0\\ 
        Ours (Simple) &1&\ding{51}&\ding{51}&0&82.6&91.5&96.5&74.8&80.2\\
        Ours (Simple with Sigmoid) &1&\ding{51}&\ding{51}&0&82.6&91.4&96.4&75.2&80.2\\
        Ours (Full, no bias)&1&0&\ding{51}&\ding{51}&80.7&90.2&96.0&72.0&78.8\\
        Ours (Full, no $k_2$)&1&\ding{51}&0&\ding{51}&80.6&87.5&91.0&73.0&78.4\\
        Ours (Full)&1&\ding{51}&\ding{51}&\ding{51}&82.4&91.4&96.7&75.3&80.2\\
         Ours (Full with Sigmoid)&1&\ding{51}&\ding{51}&\ding{51}&82.7&91.4&96.6&75.2& 80.2\\
        Ours (Full, channel-wise) &1&\ding{51}&\ding{51}&\ding{51}&82.0&91.0&96.3&74.8&80.0\\
        
			\hline
             
		\end{tabular}
		\label{tab:ablation-res}
        \vspace{-10pt}
\end{table}

\begin{table}[t]
			\caption{Impact of the parameters $k_0$, $k_1$, $k_2$ and $k_3$ of our model using the DenseNet-121 architectures in the ImageNet-to-Sketch scenario. \ding{51} denotes a learned parameter, while~$^*$ denotes \cite{mallya2018piggyback} obtained as a special case of our model.} 

		\vspace{5pt}
		\centering
		\begin{tabular}{ l | c | c | c | c | c | c | c | c | c |  } 
        Method &$k_0$ &$k_1$ & $k_2$&$k_3$& CUBS & CARS & Flowers & WikiArt & Sketch\\
         \hline
Piggyback \cite{mallya2018piggyback}&0&0&0&1&79.7&87.2&94.3&72.0&80.0\\
\hline
Piggyback$^*$ 
&0&0&0&1&80.0&86.6&94.4&71.9&78.7\\ 
Piggyback$^*$ with BN & 0&0&0&1 &81.4&90.1&95.5&73.9&79.1\\ 
Piggyback$^*$ with BN
&0&\ding{51}&0&1&81.9&90.1&95.4&72.6&79.9\\ 
        Ours (Simple, no bias)
&1&0&\ding{51}&0&80.4&91.4&96.7&75.0&79.7\\ 
        Ours (Simple) &1&\ding{51}&\ding{51}&0&81.5&91.7&96.7&75.5&79.9\\
        Ours (Simple with Sigmoid) &1&\ding{51}&\ding{51}&0&81.5&91.7&97.0&76.0&79.8\\
        Ours (Full, no bias)&1&0&\ding{51}&\ding{51}&80.2&91.1&96.5&75.1&79.2\\
        Ours (Full, no $k_2$)&1&\ding{51}&0&\ding{51}&79.8&87.2&91.8&73.2&78.1\\
        Ours (Full)&1&\ding{51}&\ding{51}&\ding{51}&81.7&91.6&96.9&75.7&79.9\\
         Ours (Full with Sigmoid)&1&\ding{51}&\ding{51}&\ding{51}&82.0&91.7&97.0&76.0&79.9\\
        Ours (Full, channel-wise) &1&\ding{51}&\ding{51}&\ding{51}&81.4&91.6&96.5&75.5&79.9\\
        
			\hline
             
		\end{tabular}
		\label{tab:ablation-dense}
        \vspace{-10pt}
\end{table}
