# Supplementary material for: Boosting Binary Masks for Multi-Domain Learning through Affine Transformations
Source: arXiv:2103.13894 source file (2021-03-25)
Supplement: Supplementary file 2 [file parameters.tex]

In this section we re-propose the parameter analysis of the main paper, reporting the results for all the datasets (in a clearer graphical form). Also for the remaining datasets (\ie WikiArt and Sketch) the plots show similar trends as for the other datasets, both in term of active weights, density of the masks and value of the parameters $k_1$,$k_2$ and $k_3$. In fact, also in these datasets, our model has a sparser and more constant number of active masks across the whole architectures, with respect to the ones obtained by Piggyback. We also note that the values of $k_2$ and $k_3$ reach larger magnitudes compared to $k_1$, with $k_1$ and $k_2$ usually having a different sign. Moreover, the fact that weight transformations are more remarked as depth increases is even more evident for WikiArt and Sketch due to the variability that these datasets contain with respect to standard natural images.%In all scenarios our model keeps almost half of the masks active across the whole architecture. Compared to the masks obtained by Piggyback, there are 2 differences: 1) Piggyback exhibits denser masks (\ie with a larger portion of 1s), 2) the density of the masks in Piggyback tends to decreases as the depth of the layer increases. Both these aspects may be linked to the nature of our model: by having more flexibility through the affine transformation adopted, there is less need to keep active large part of the network, since a loss of information can be recovered through the other components of the model, as well as constraining a particular part of the architecture. For what concerns the value of the parameters $k_1$, $k_2$ and $k_3$ for both architectures $k_2$ and $k_3$ tend to have larger magnitudes with respect to $k_1$. Also, the values of $k_2$ and $k_1$ tend to have a different sign, which allows the term $k_1\mat 1+k_2\mat M$ to span over positive and negative values. We also notice that the transformation of the weights are more prominent as the depth increases, which is intuitively explained by the fact that baseline network requires stronger adaptation to represent the higher-level concepts pertaining to different tasks.

\begin{figure}[!b]
\centering
%   \subfloat[asda]{\label{fig:bn}
 \includegraphics[width=1.\textwidth,trim=2cm 0 1.5cm 0,clip]{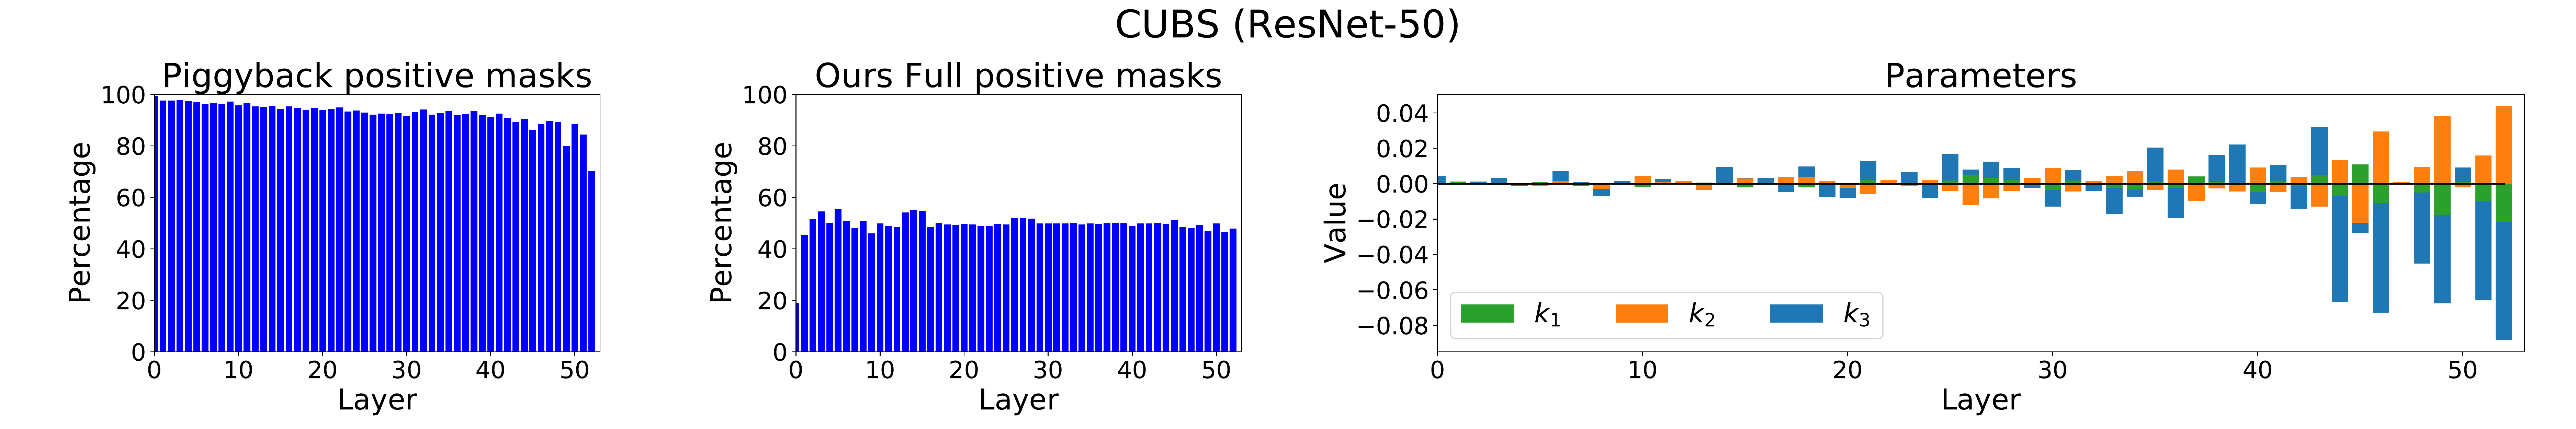}  \\
%   }\\
%   \subfloat[asda]{\label{fig:da-bn}
\includegraphics[width=1.\textwidth,trim=2cm 0 1.5cm 0,clip]{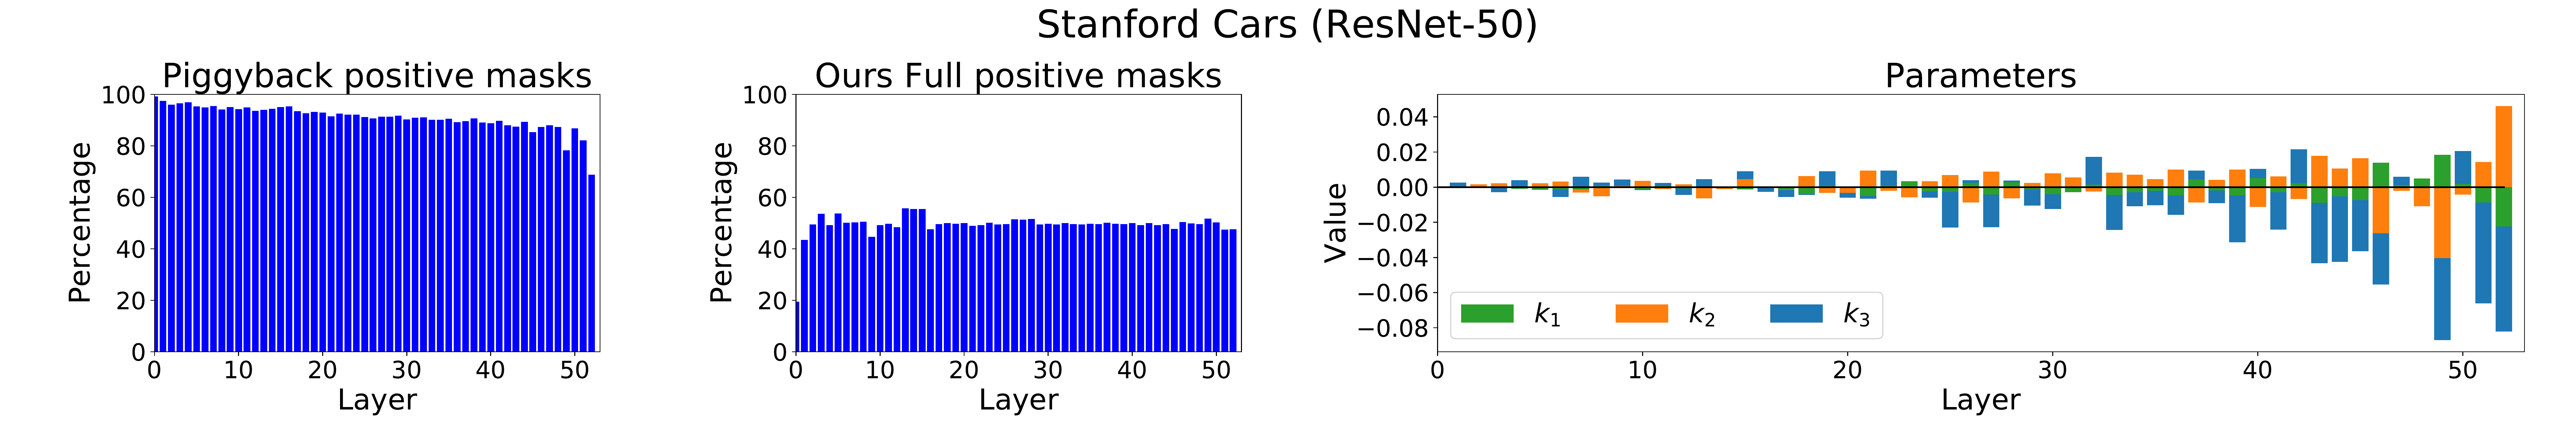} \\
%   }\\
%   \subfloat[asda]{\label{fig:da-bn}
\includegraphics[width=1.\textwidth,trim=2cm 0 1.5cm 0,clip]{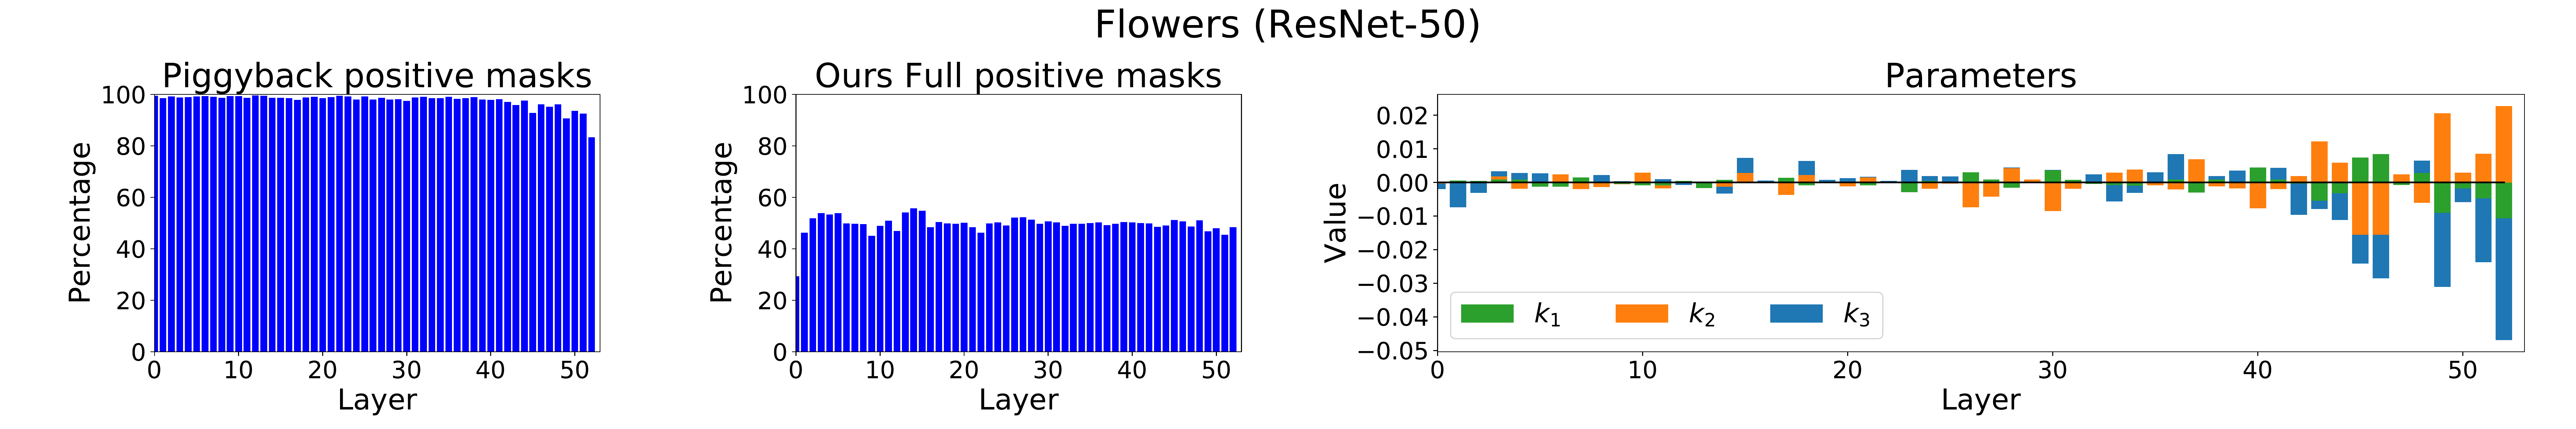} \\
%   }\\
%   \subfloat[asda]{\label{fig:da-bn}
\includegraphics[width=1.\textwidth,trim=2cm 0 1.5cm 0,clip]{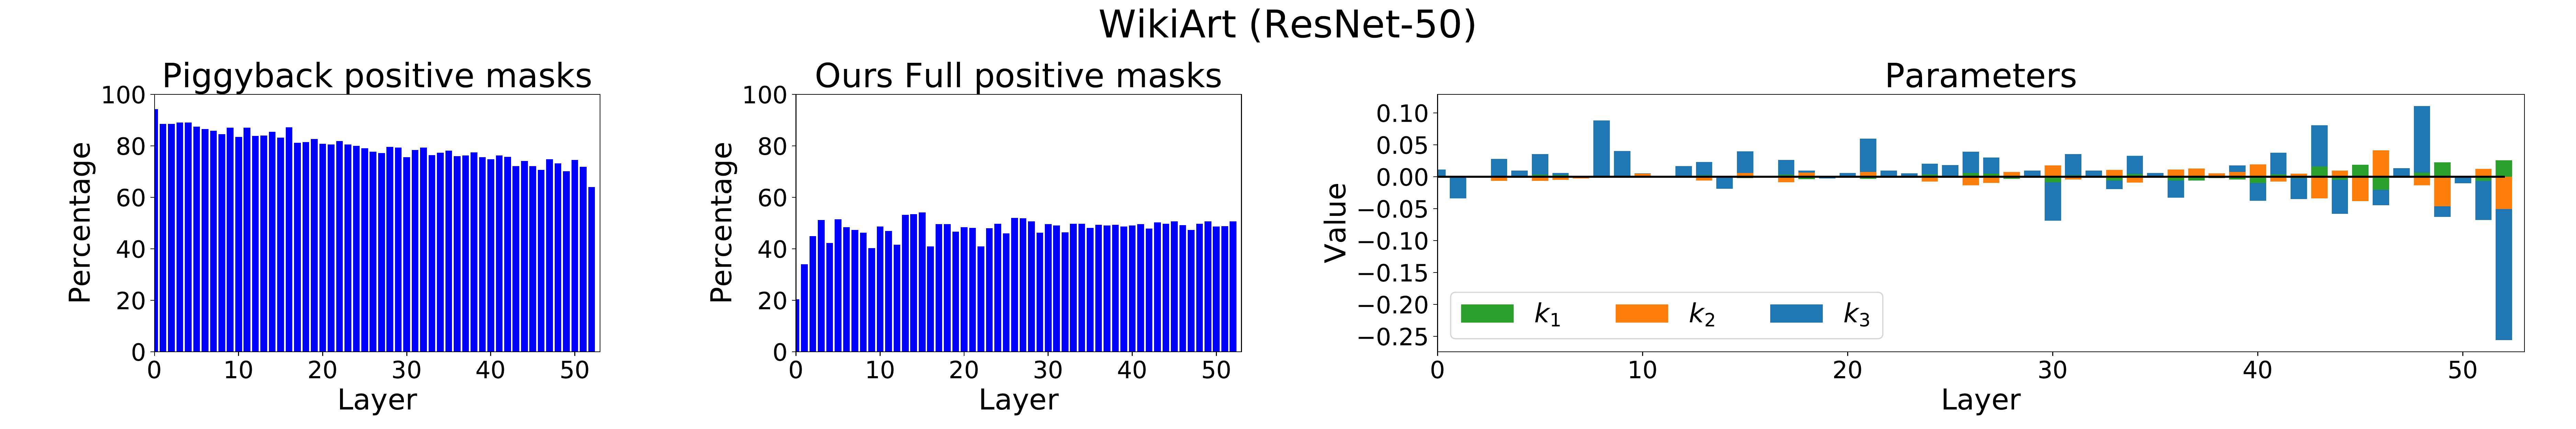} \\
%   }\\
%   \subfloat[asda]{\label{fig:da-bn}
\includegraphics[width=1.\textwidth,trim=2cm 0 1.5cm 0,clip]{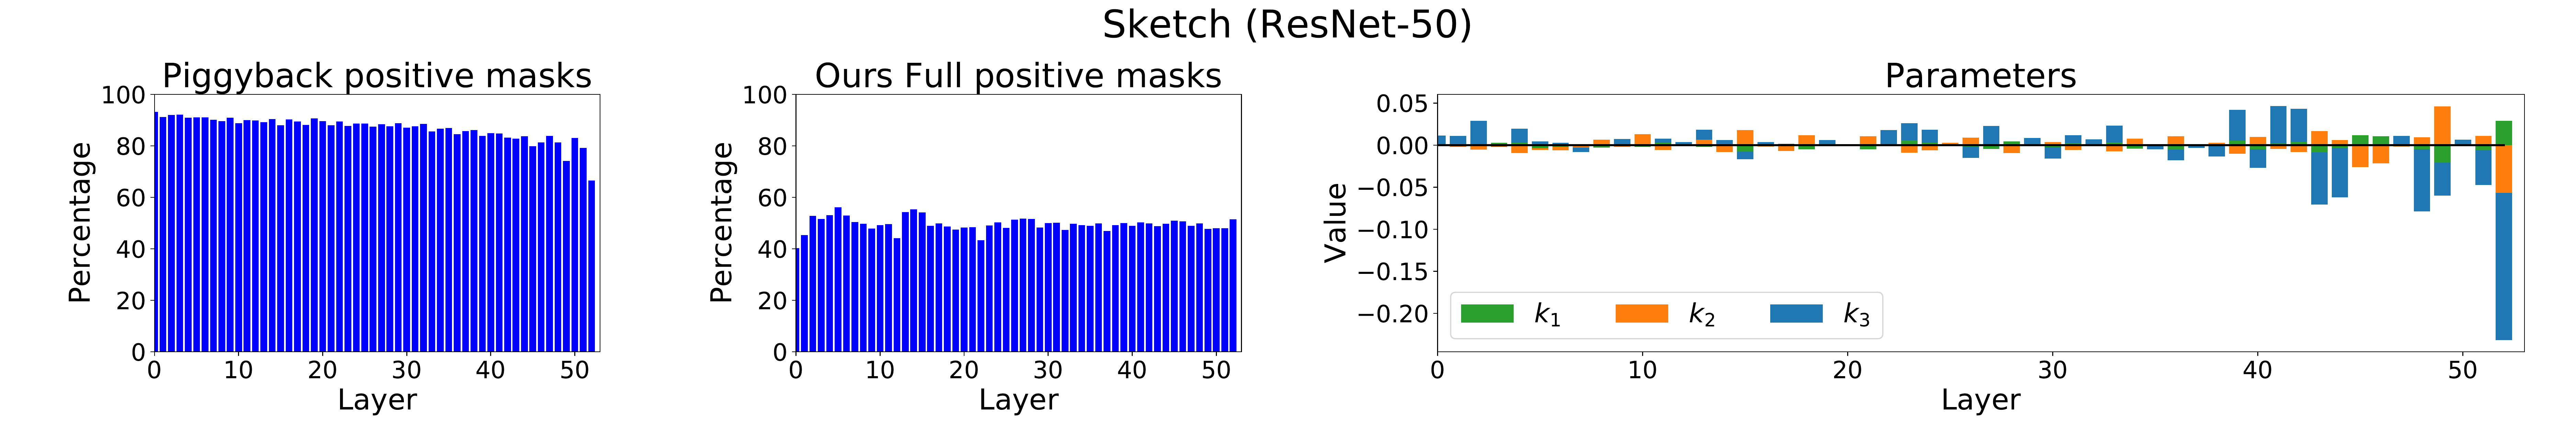} \\
   %}
  \caption{Percentage of 1s in the binary masks at different layers depth for Piggyback (left) and our full model (center) and values  of the parameters $k_1$, $k_2$, $k_3$ computed by our full model (right) for all datasets of the Imagenet-to-Sketch benchmark and the ResNet-50 architecture.
  }
  \end{figure}

  \begin{figure}[!b]
\centering
%   \subfloat[asda]{\label{fig:bn}
   \includegraphics[width=1.\textwidth,trim=2cm 0 1.5cm 0,clip]{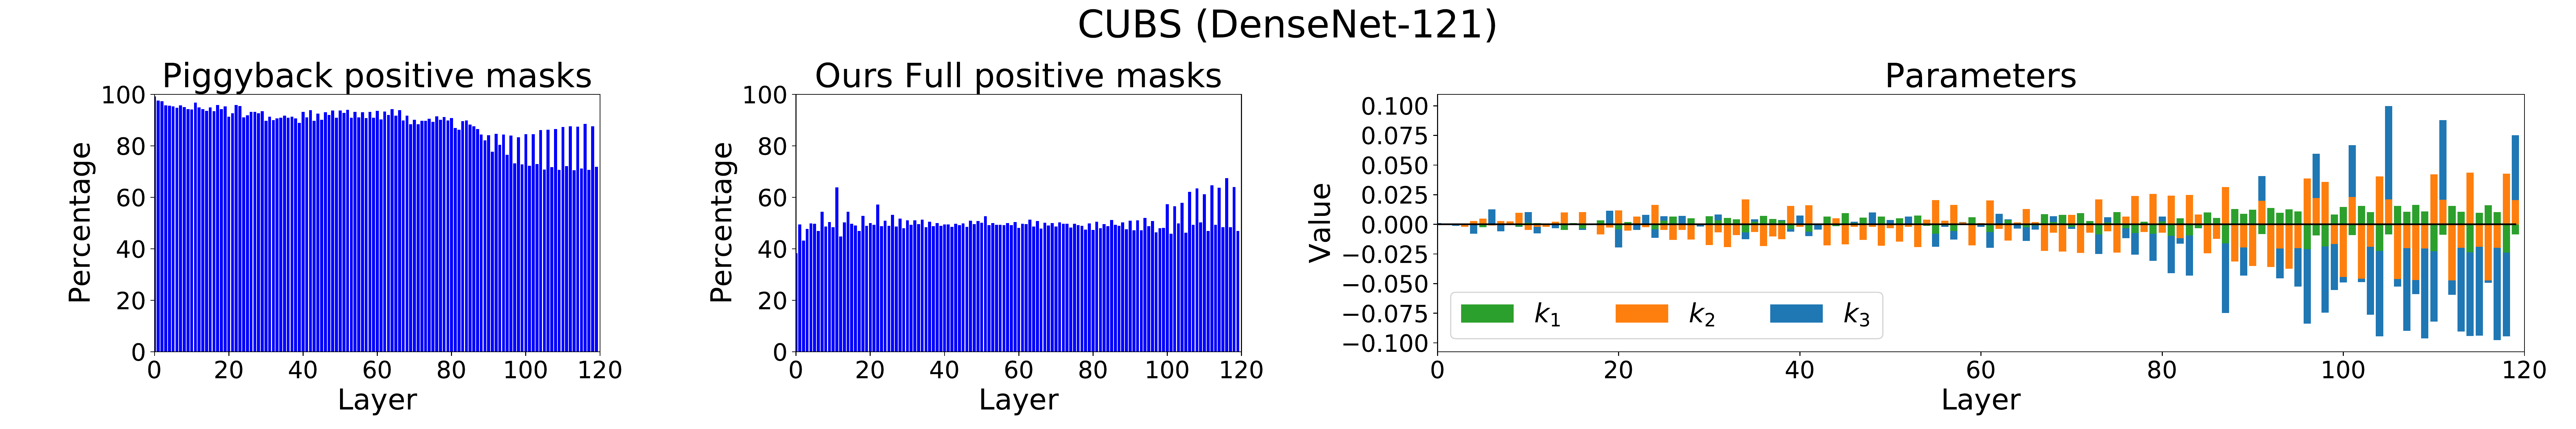}  \\
%   }\\
%   \subfloat[asda]{\label{fig:da-bn}
\includegraphics[width=1.\textwidth,trim=2cm 0 1.5cm 0,clip]{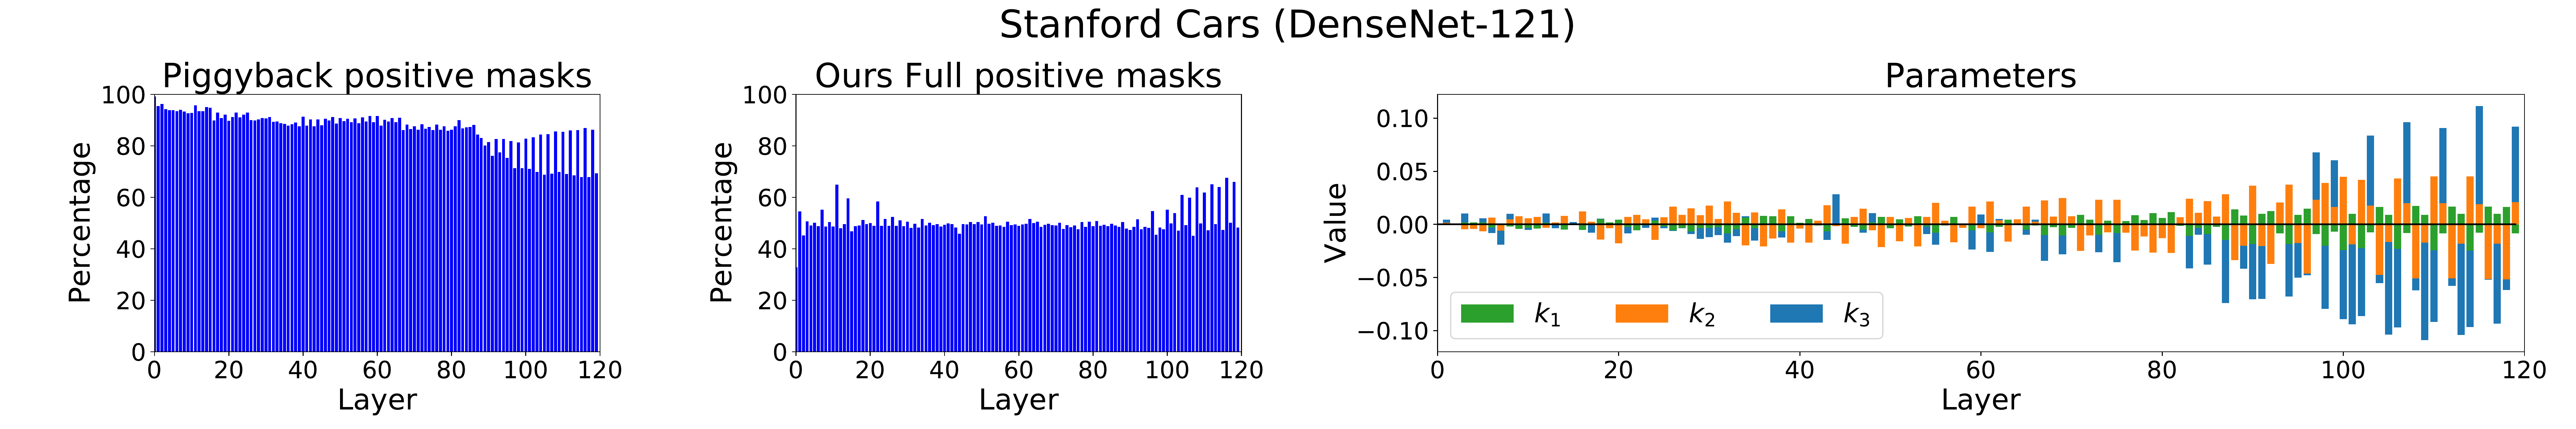} \\
%   }\\
%   \subfloat[asda]{\label{fig:da-bn}
\includegraphics[width=1.\textwidth,trim=2cm 0 1.5cm 0,clip]{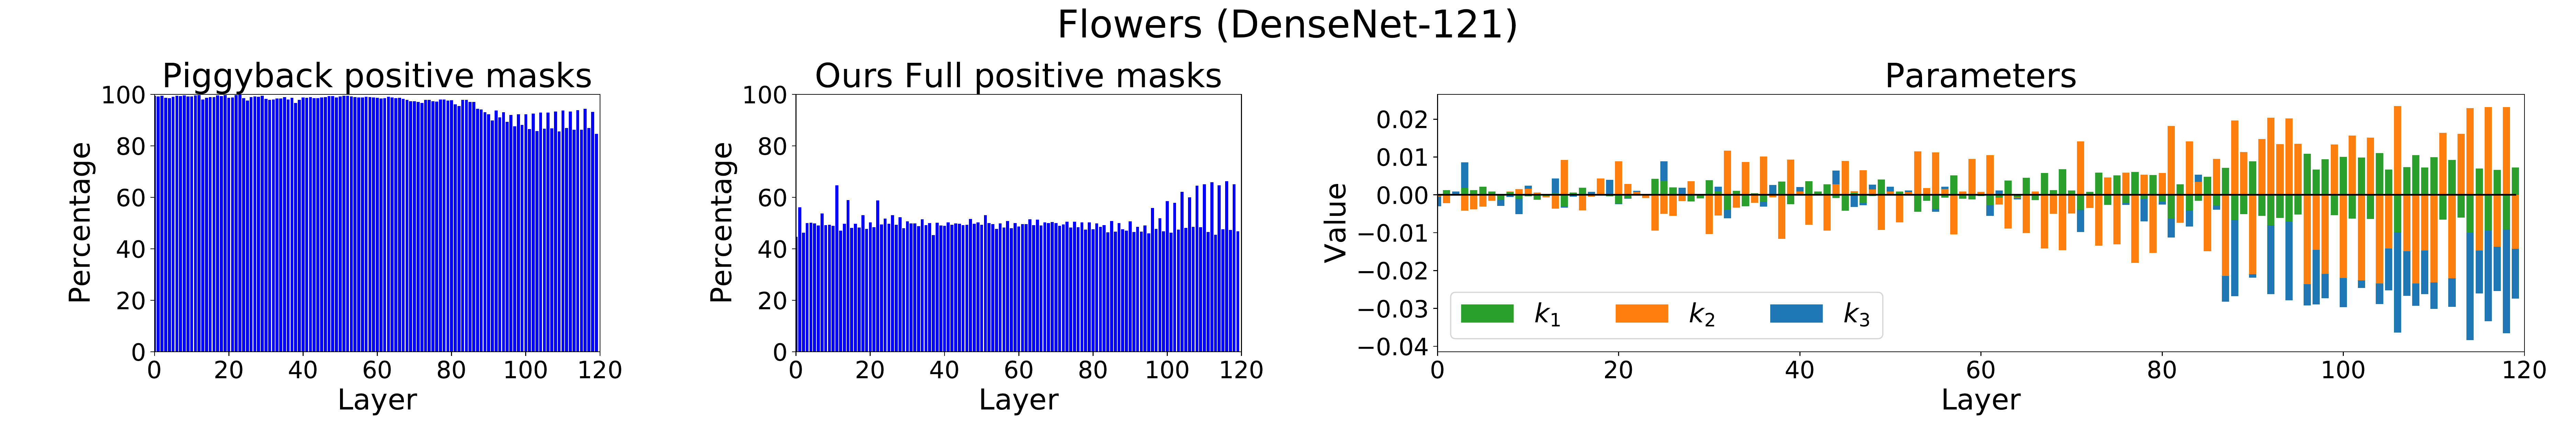} \\
%   }\\
%   \subfloat[asda]{\label{fig:da-bn}
\includegraphics[width=1.\textwidth,trim=2cm 0 1.5cm 0,clip]{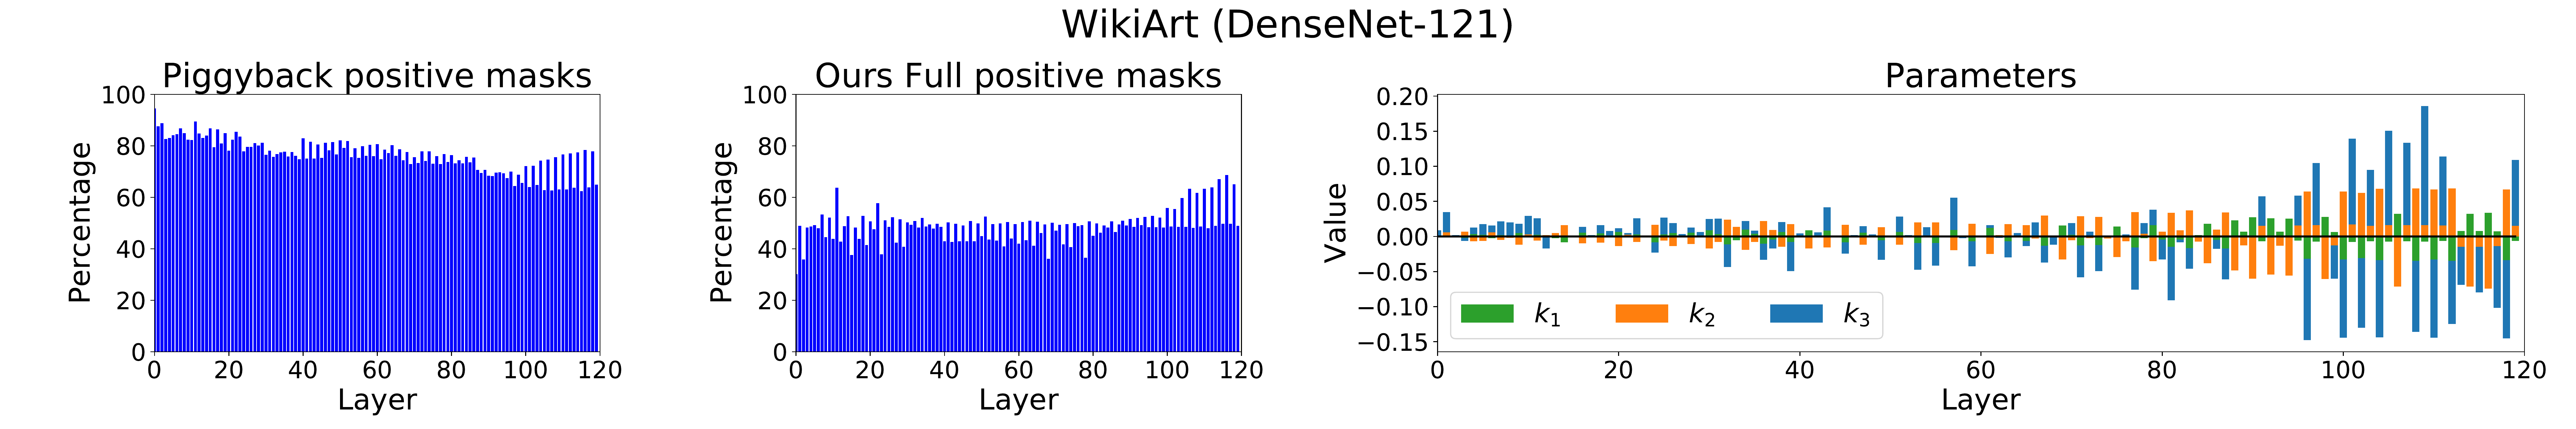} \\
%   }\\
%   \subfloat[asda]{\label{fig:da-bn}
\includegraphics[width=1.\textwidth,trim=2cm 0 1.5cm 0,clip]{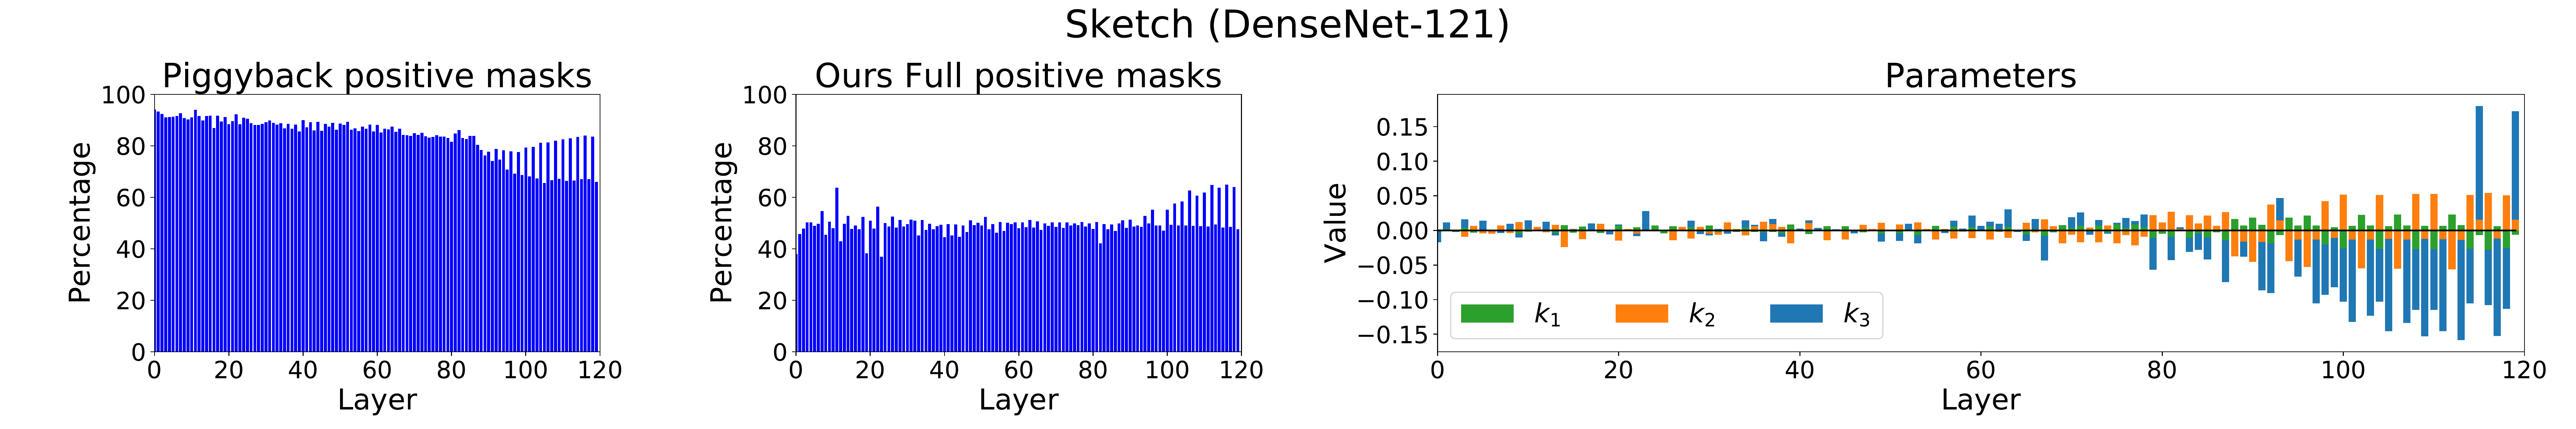} \\
   %}
  \caption{Percentage of 1s in the binary masks at different layers depth for Piggyback (left) and our full model (center) and values  of the parameters $k_1$, $k_2$, $k_3$ computed by our full model (right) for all datasets of the Imagenet-to-Sketch benchmark with the DenseNet-121 architecture.
  }
  \end{figure}
